# Supplementary material for: Counterfactual States for Atari Agents via Generative Deep Learning
Source: arXiv:1909.12969 source file (2019-09-27)
Supplement: Supplementary file 1 [file supplementary.tex]

\subsection{Architecture and Training}

The pre-trained agent is a convolutional feed-forward network that takes a set of 4 concatenated monochrome frames as input and is trained to maximize game score using the Asynchronous Advantage Actor-Critic (A3C) algorithm \cite{Mnih15}.
The frames are down sampled and cropped to 80x80, with normalized values [0,1]. This input is processed by 4 convolutional layers (each with 32 filters, kernel sizes of 3, strides of 2, and paddings of 1), followed by a fully connected layer, sized 256, and a last fully connected layer size $|A| + 1$, where $A$ is the action space size. We apply a softmax activation to the first $|A|$ neurons to obtain $\pi(s)  = a$ and use the last neuron to predict the value, $V(s)$. 

The A3C RL algorithm was trained with a learning rate of $\alpha = 10^{-4}$ , a discount factor of $\gamma = 0.99$, and computed loss on the policy using Generalized Advantage Estimation with $\lambda = 1.0$. We find that convergence is more difficult with such a large frame skip, so each policy was trained asynchronously for a total of 160 million frames.

During training, we do not downscale or greyscale the game state. We pass in the current game time step, along with the previous 3 time steps, stacked together for a total of 12 channels: 4 game steps each with 3 channels, RGB.

\subsubsection*{Encoder Network}
The Encoder $E$ consists of the following layers.
\begin{enumerate}
\item
 Input 12 channels size 160x160, kernel size 3, output 32 channels.
\item
 Kernel size 3, output 64 channels.
\item
 Kernel size 4, output 128 channels.
\item
 Kernel size 4, output 256 channels.
\item
 Kernel size 4, output 256 channels.
\item
 Kernel size 3, output 256 channels.
\item
Fully connected layer from 3x3x256 to 16.
\end{enumerate}
All but the last layer have padding of size 1 and a stride of 2.
The last layer has no padding and a stride of 1.
All convolutional layers are followed by batch normalization and the non-linearity function leaky ReLU with a leak of $0.2$.
The output of the network is referred to in the text as $E(s)$.

\subsubsection*{Generator Network}
The Generator $G$ consists of the following:
\begin{enumerate}
\item
Fully connected layer that takes as input $E(s)$ concatenated with the agent's output $\bm{\pi}(z)$, where $z = A(s)$
\item
Transposed convolution, outputs 512 channels.
\item
Transposed convolution, outputs 256 channels.

\item
Transposed convolution, outputs 128 channels.

\item
Transposed convolution, outputs 128 channels.

\item
Transposed convolution, outputs 64 channels.

\item
Transposed convolution, outputs 12 channels.
\end{enumerate}

Each layer after the first is a transposed convolution with stride of 2, kernel size of 4, and takes as input the previous layer's output concatenated with $\bm{\pi}(s)$ as additional constant input channels.
Each layer except the last one is followed by batch normalization and the ReLU function.
The last layer is followed the sigmoid function.

\subsubsection*{Discriminator Network}
The Discriminator D consists of the following:
2 fully connected layers the same size as the input $E(s)$. 
%lwneal suggestion: a Dropout layer with p=0.2, with dropout applied during training and disabled during evaluation.
Each layer is followed by a dropout layer of $0.2$ and a leaky ReLU non-linearity with a leak of $0.2$.
And a 3rd fully connected layer the that outputs the size of the actions $|A|$. This layer is then followed by a softmax function.

These 3 networks are all trained through stochastic gradient descent with the Adam optimizer, with parameters $\alpha = 1^{-4}, \beta_{1} = 0, \beta_{2} = .9$. These networks were typically trained for 40 million game states to achieve high fidelity reconstructions, but we found 10 million (or even 2.5 million) game states to be enough to produce meaningful counterfactual states.

\subsubsection*{Wasserstein Autoencoder}
The Wasserstein encoder $E_w$ consists of 3 fully-connected layers mapping $\bm{z}$ to a 128-dimensional vector $\bm{z}_w$, normalized such that $||z_w|| = 1$. Each layer has the same dimensionality of 256, except the output of the 3rd layer which is 128. Additionally, the first two layers are followed by batch normalization and leaky ReLU with a leak of $0.2$.

The corresponding Wasserstein decoder $D_w$ is symmetric to $E_w$, with batch normalization and leaky ReLU after the first two layers and maps $\bm{z}_w$ back to $\bm{z}$.

The Wasserstein Autoencoder was trained with Adam optimizers of the same learning rate $\alpha = 1^{-4}$ and with the default $\beta$ parameters. Training was performed for 15 million frames, upon which we found selecting actions from $\bpi(D_w(E_w(A(\bs))))$ were close to the scores of the original agent (at most $0.25$ of a standard deviation away).

\subsection{Ablation Experiments}

\begin{figure*}[t]
    \centering
   \includegraphics[width=.19\linewidth]{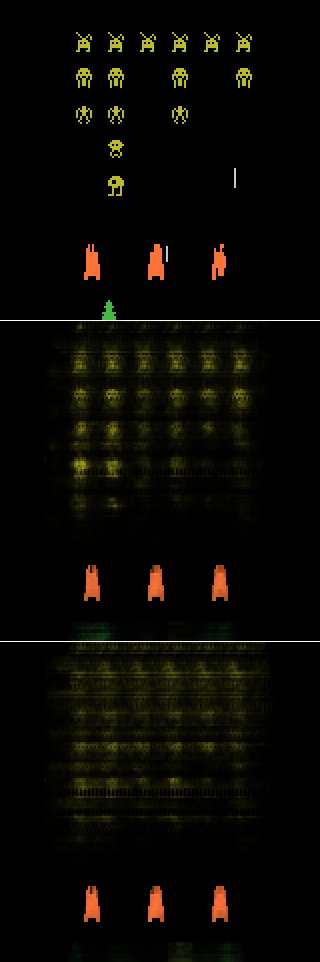}
   \includegraphics[width=.19\linewidth]{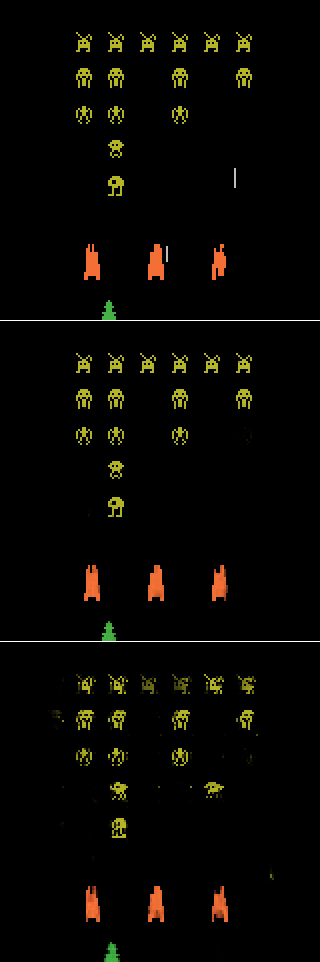}
    \includegraphics[width=.19\linewidth]{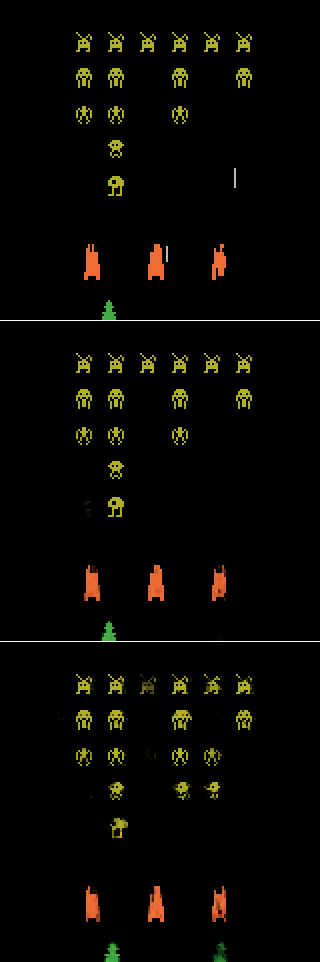}
    \includegraphics[width=.19\linewidth]{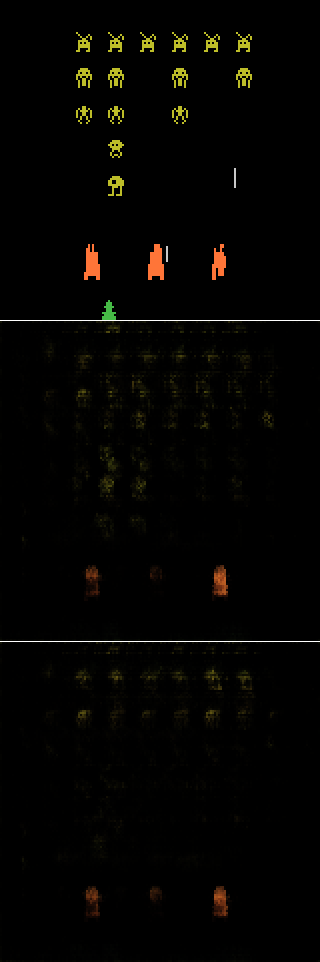}
    \includegraphics[width=.19\linewidth]{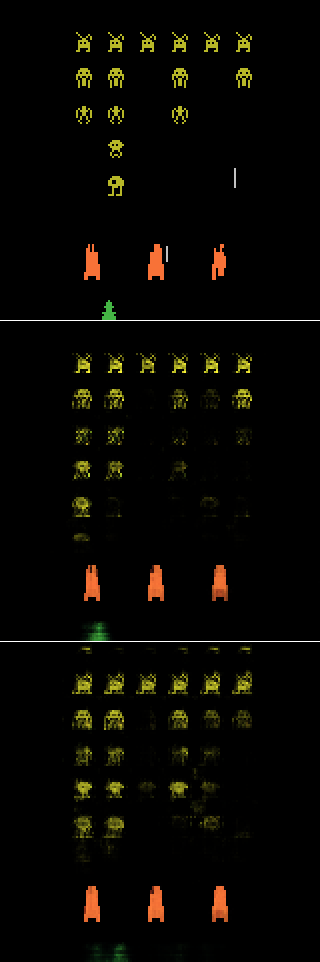}
    \caption{From left to right: ablations 1 - 5.  In each column, (\textbf{top}) image is the original state where $a =$ \textit{MoveRight}, (\textbf{center}) the auto-encoded reconstruction of the original state, (\textbf{bottom}) is a counterfactual state where $a'=$ \textit{MoveRightAndFire}.}
    \label{fig:ablations1}    
\end{figure*}

\begin{table}[]
\begin{tabular}{l||l|l|l|l}
Ablation experiment & $E(s)$ & $z_w$ & $z$ & $\bpi(A(\bs))$  \\ \hline \hline
1  &                &              &                & \checkmark     \\ \hline
2  &                &              & \checkmark     &                \\ \hline
3  &                &              & \checkmark     & \checkmark     \\ \hline
4  &                & \checkmark   &                &                \\ \hline
5  &                & \checkmark   &                & \checkmark     \\ \hline
6  & \checkmark     &              &                & \checkmark     \\ \hline
7  & \checkmark     &              & \checkmark     &                \\ \hline
8  & \checkmark     &              & \checkmark     & \checkmark     \\ \hline
9  & \checkmark     & \checkmark   &                &                \\ \hline
10 & \checkmark     & \checkmark   &                & \checkmark      
\end{tabular}
\caption{An overview of what elements are given as input to the generator for each ablation experiment.}
 \label{table:ablations}
\end{table}

For all ablation experiments we use the same architecture as described above. A generator is always used with MSE reconstruction loss, but what we pass into the generator changes for each ablation experiment. We provide an overview of the different ablations in Table \ref{table:ablations} and Figures \ref{fig:ablations1} and \ref{fig:ablations2} contain images which are representative of the issues for each ablation experiment.

\begin{figure*}[t]
    \centering
    \includegraphics[width=.19\linewidth]{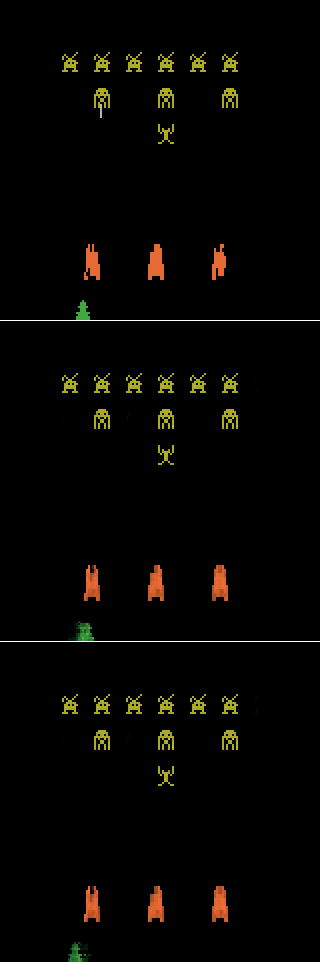} 
    \includegraphics[width=.19\linewidth]{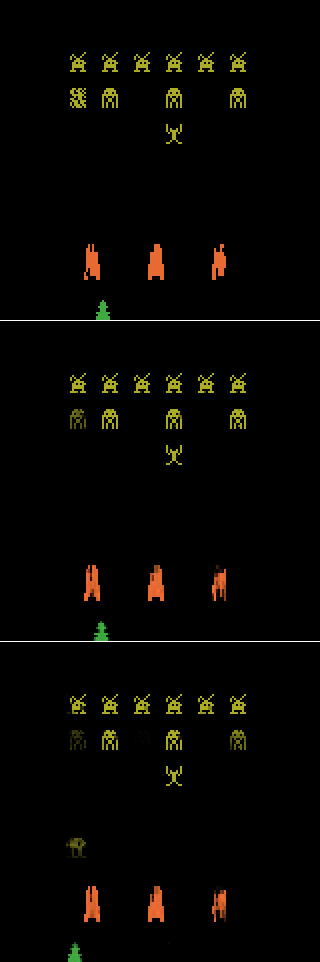}
    \includegraphics[width=.19\linewidth]{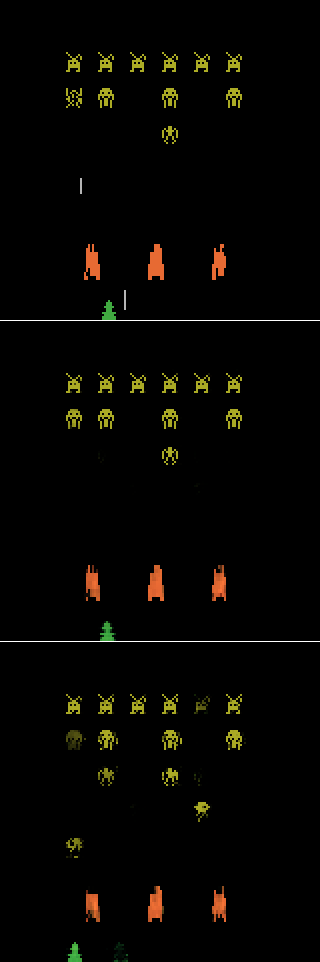}
    \includegraphics[width=.19\linewidth]{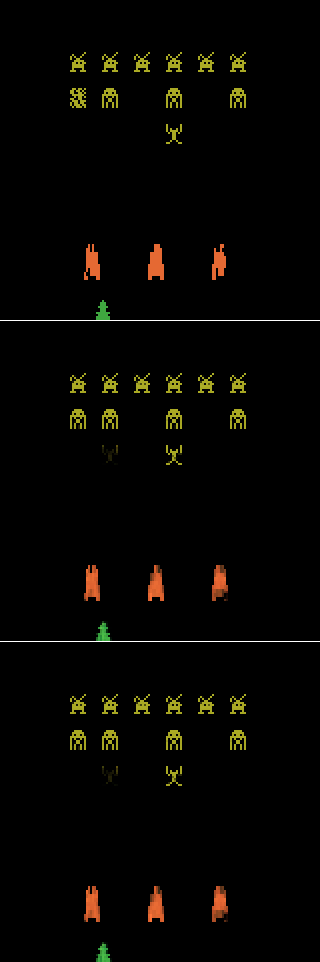}
    \includegraphics[width=.19\linewidth]{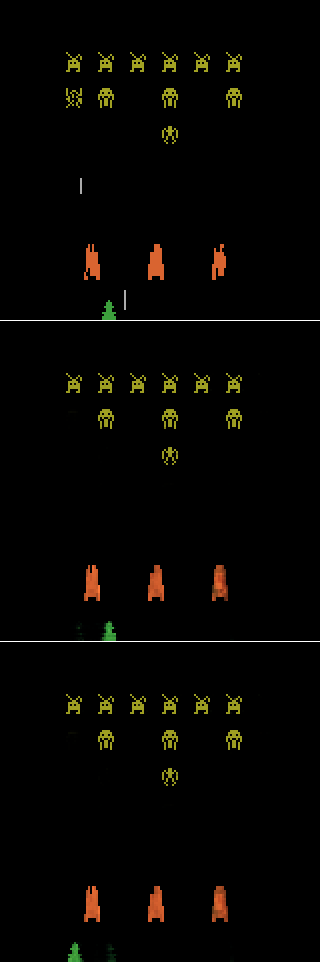}
    \caption{From left to right: ablations 6 - 10. In each column, the top image is an original state where $a =$ \textit{MoveRight}, the middle image is an auto-encoded reconstruction, and the bottom is a counterfactual state where $a'=$ \textit{MoveRightAndFire}.}
    \label{fig:ablations2}
\end{figure*}

\begin{enumerate}
    %1
    \item  For this ablation, we investigate the effect of only using the agent's policy to generate reconstructed states and hand-modifying it to create counterfactual states: removing all parts from our model except the agent and the generator, passing solely the $\bpiz$, where $\bz = A(\bs)$, into the generator. This gives us reconstructed states in the form of $G(\bpiz)$. We modify the policy vector $\bpiz$ by selecting a counterfactual action $a'$, setting $\bpi(\bz,a') = \bpiza * 1.01$, and normalizing the probabilities back to 1. This hand modification is clearly not representative of the agent. As shown in figure \ref{fig:ablations1}, the reconstructed and counterfactual states are extremely low quality. 
    %2
    \item For this ablation, we investigate the effect of only using the agent's learned representation to generate both reconstructed states and counterfactual states. We removed all parts from our model except the agent and the generator, passing $\bm{z}$ into the generator. This gives us reconstructed states in the form of $G(\bz)$ and counterfactual states by modifying $\bz$ with gradient descent as described in section \ref{sec:generating_counterfactuals} to get a $\bm{z}^*$. As shown in figure \ref{fig:ablations1}, the counterfactual states are quite unrealistic, but surprisingly the reconstructed states are accurate. %\hl{should we write more here and suggest further analysis could be done?}
    %3
    \item For this ablation, we removed all parts from our model except the agent and the generator, this time passing both $\bz$ and $\bpiz$ into the generator. This gives us reconstructed states in the form of $G(\bz,\bpiz)$ and counterfactual states by modifying $\bz$ with gradient descent as described in section \ref{sec:generating_counterfactuals} to get a $\bm{z}^*$. As shown in figure \ref{fig:ablations1}, the counterfactual states are quite unrealistic, but surprisingly the reconstructed states are accurate.
    %4
    \item For this ablation, we investigate using only the Wasserstein auto-encoder. Here we pass only $\bzw$ into the generator, where $\bzw$ is the latent representation of the state in Wasserstein space $\bzw = E_w(A(\bs))$. This gives us reconstructed states in the form of $G(\bzw)$ and counterfactual states by modifying $\bzw$ with gradient descent as described in section \ref{sec:generating_counterfactuals} to get a $\bm{z_w}^*$. As shown in figure \ref{fig:ablations1}, both the reconstructed and counterfactual states are quite unrealistic.
    %5
    \item For this ablation, we removed all parts from our model except the agent, the Wasserstein auto-encoder, and the generator. Here we pass both $\bzw$ and $\bpiz$ into the generator. This gives us reconstructed states in the form of $G(\bz,\bpiz$) and counterfactual states by modifying $\bzw$ with gradient descent as described in section \ref{sec:generating_counterfactuals} to get a $\bm{z_w}^*$. As shown in figure \ref{fig:ablations2}, both the reconstructed and counterfactual states improve relative to the previous ablation, but are still quite unrealistic.
    %6
 %   \item This is equivalent to a simple autoencoder, as the loss of removing anything from the latent space . You could in theory manipulate the latent space with respect to the agent, but that's not representative of the agent, only pixel space (ie, similar states in pixel space != similar in true game space) (e.g. entering a death animation), also the Agent takes 80x80 monochrome, so your AE would have to accommodate for that...\hl{This ablation is so weird compared to the other methods, that even though it was our previous research from the summer, I don't think we need to keep it.}
    %I doubt a reviewer would see all 10 other ablations and think, "but what if they used a VAE and modified the latent space, then sent the output image through the agent to generate CFs"
    %7
    \item
    %This seems to work and produces good counterfactual states, but here we manually modify the probabilities. 
    
    For this ablation, we investigate the effect of keeping the encoder and discriminator, but hand-modify the policy input to the generator instead of using the Wasserstein auto-encoder or gradient descent. The input to the generator is equivalent to our work described in section 3. We hand-modify the policy vector $\bpiz$, by selecting a counterfactual action $a'$, setting $\bpi(\bz,a') = \bpiza * 1.01$, and normalizing the probabilities back to 1. These hand modification may, or may not, be representative of the agent. As shown in figure \ref{fig:ablations1}, the states have the same generated quality as our method and the counterfactual state has a small, but meaningful change.  
    %8
    \item% better than no fader, but the counterfactuals are still bad
    
    This ablation is similar to the previous, but instead of passing the policy vector $\bpiz$ to the generator, we input the agent's latent space $\bz$.
    As with previous ablations, we generate counterfactual states by modifying $\bz$ with gradient descent as described in section \ref{sec:generating_counterfactuals} to get a $\bm{z}^*$. As shown in figure \ref{fig:ablations2}, the states have a decent quality, but the counterfactual states have relatively large changes and a couple of artifacts.  
    %9
    \item %better than no labels, but the counterfactuals aren't very good 
    
    This ablation is similar to the previous, but instead of passing just $\bz$, we pass in both the policy vector $\bpiz$ and $\bz$ to the generator.
    As with previous ablations, we generate counterfactual states by modifying $\bz$ with gradient descent as described in section \ref{sec:generating_counterfactuals} to get a $\bm{z}^*$. As shown in figure \ref{fig:ablations2}, the states are better quality than just passing in $\bm{z}^*$, but the counterfactual are lower quality than our method.  
    %10
    \item %little to no change between the reconstructed state and the counterfactual state 
    
    In this ablation, we add back in the Wasserstein auto-encoder. Instead of passing in the agent's latent space $\bz$ to the generator, we pass in the Wasserstein representation $\bzw = E_w(A(\bs))$.
    As described in \ref{sec:generating_counterfactuals}, we generate counterfactual states by modifying $\bzw$ to get a $\bm{z_w}^*$. As shown in figure \ref{fig:ablations2}, the states are high quality, but the counterfactual states typically have no changes.  
    %11
    \item This experiment is an ablation in the sense that we remove the disconnection between the generation and $\bzw$. In other words, we take our original method and add $\bzw$ as input to the generator. When counterfactual states are generated, $\bm{z_w}^*$ is passed into the generator along with $E(\bs)$ and $\bm{\pi}(\bm{z_w}^*)$. As shown in figure \ref{fig:ablations2}, the states are high quality and the counterfactual states are interesting. We were not able to find a difference in quality for generated states between this ablation and our method. Since this ablation is more complex, and requires more parameters, we decided not to use it for our purposes.
\end{enumerate}

\subsection{Additional counterfactual state examples}

%use seaquest ex 3 here. a = upleft shoot, a' = upleft
%use the 3 crazy climber examples
\paragraph{Crazy Climber}
In this game, an agent must climb up a building while avoiding various obstacles. 
Figure \ref{fig:crazy_climber} (\textbf{Left, Center}) show how the agent understands the different levels of climbing animations. Figure \ref{fig:crazy_climber} (\textbf{Right}) shows how the agent will avoid the large open areas, but also shows a failure state of not producing the enemy. It is not clear if this is due to our model, or simply because the agent never learns to avoid any enemies during normal play and our model captures this.

\begin{figure*}[t]
    \centering
    \includegraphics[width=\linewidth]{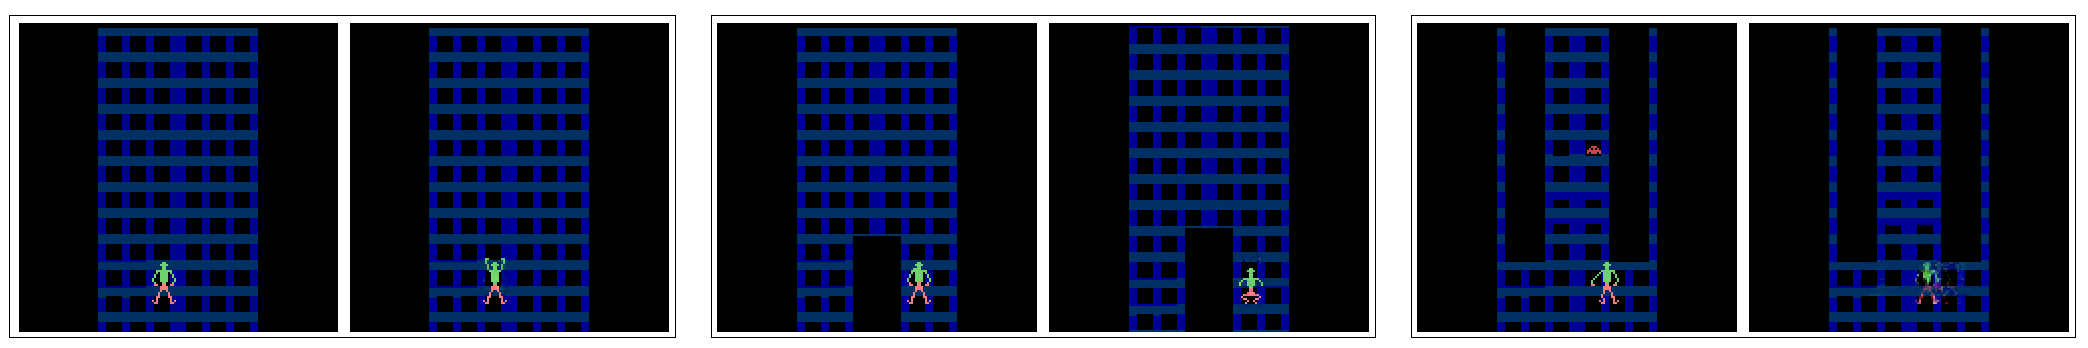}
    \caption{Example query state (left) and counterfactual state (right) pairs for Crazy Climber. \textbf{Left}: $a =$ \textit{Up}, $a'=$ \textit{Down}.    \textbf{Center}: $a=$ \textit{Up}, $a'=$ \textit{Down}.    \textbf{Right:} $a=$ \textit{Left}, $a'=$ \textit{Up}, where $a$ is the query state and $a'$ is the counterfactual action.
    }
   
    \label{fig:crazy_climber}
\end{figure*}

\paragraph{A full counterfactual example}
When training the agent and our model, we use the current time step and previous 3 time steps concatenated as input. In Figure \ref{fig:full_space_invader}, we show what the full state and counterfactual state look like. We found it much more clear to simply show the current time step than show the frame history.

\begin{figure}[t]
    \centering
    \includegraphics[width=\columnwidth]{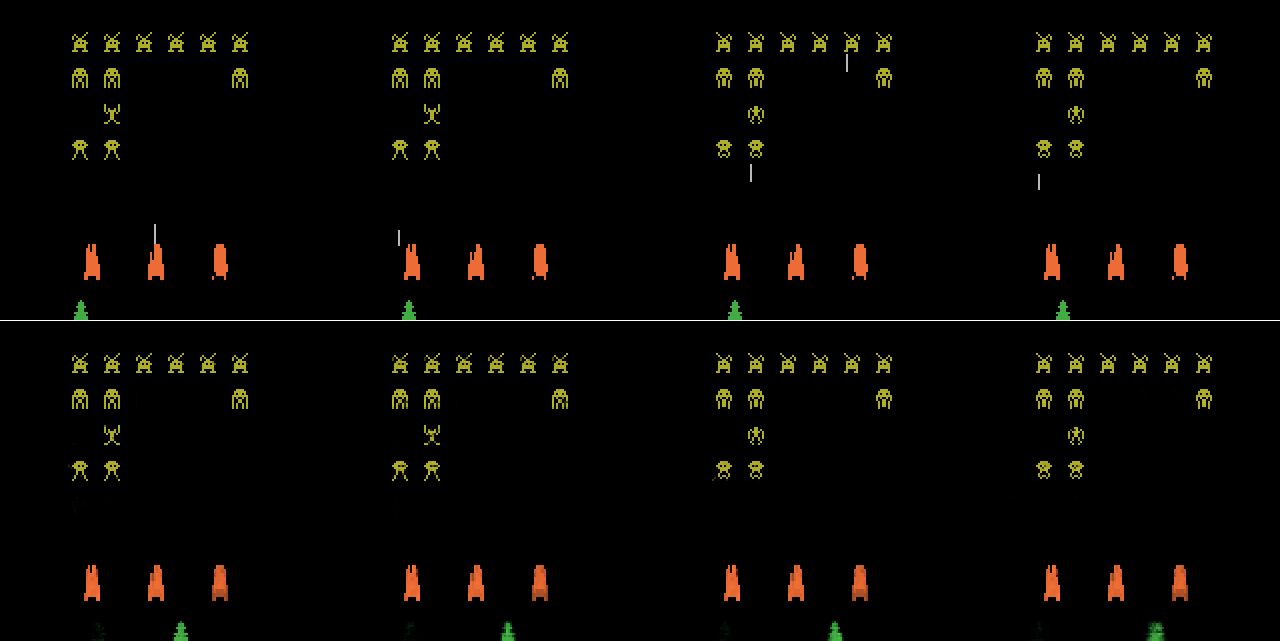}
    \caption{(\textbf{Top}): the full original state $a = $ \textit{MoveRight}. (\textbf{Bottom}): the full counterfactual state $a' = $ \textit{Fire}. The rightmost column is the current time-step in the game, where each previous column is an additional time-step in the past.}
   
    \label{fig:full_space_invader}
\end{figure}

\subsection{Baseline Experiment}
Here we investigate a baseline method that doesn't use any generative methods: nearest neighbors. We run our pre-trained agent for 1 million game steps, $M$, with $\epsilon$-greedy exploration. For each step we store, in a set $\mathcal{N}$, the state $\bs$, the representation $\bz = A(\bs)$, and the action taken $a$; this gives us a dataset $\mathcal{N} = \{(\bm{s}_1, \bz_1, a_1), \ldots, (\bm{s}_M, \bz_M, a_M))$. To generate a counterfactual, we let the agent play a new game, and on the desired state $\bs$ we find the nearest, $L_2$, latent point $\bz^* \in \mathcal{N}$ to the current point $A(\bs)$ where the agent takes the desired action of $a'$. We can then display the associated state $\bs^*$ as the closest, counterfactual, state where the agent takes a different action $a'$. 

We find that the results of nearest neighbor produce counterfactuals of inconsistent quality. Some of the results do fit our definition of counterfactual and provide meaningful insight into the agent. Other results have odd changes in the state, for example an extra alien appearing on the opposite side from the agent for seemingly no reason. And lastly, some results are extremely different from the current state and certainly do not fit our definition of closeness for a counterfactual: either a reset of the game or many enemies being added/removed. We show some representative counterfactuals for this method in \ref{fig:nearest_neighbors}; we include the image highlight for the subtle, and not so subtle, changes.

\begin{figure*}[t]
    \centering
    \begin{subfigure}{0.49\textwidth}
        \centering
        \includegraphics[width=\textwidth]{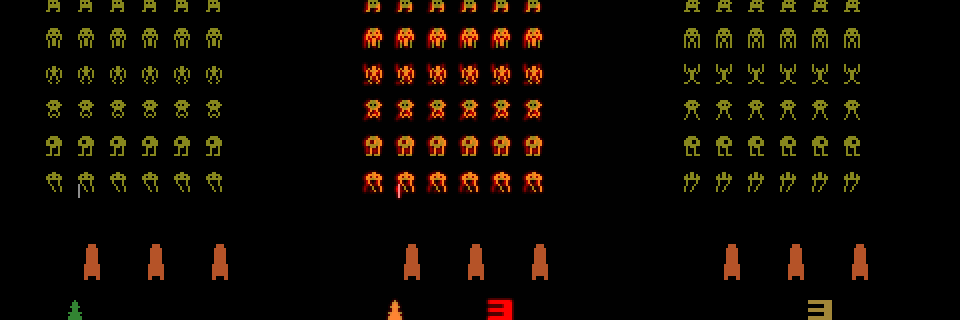}
        \caption{$a =$ \textit{MoveRightAndFire}, $a'=$ \textit{MoveLeft}.}
    \end{subfigure}%
    ~ 
    \begin{subfigure}{0.49\textwidth}
        \centering
        \includegraphics[width=\textwidth]{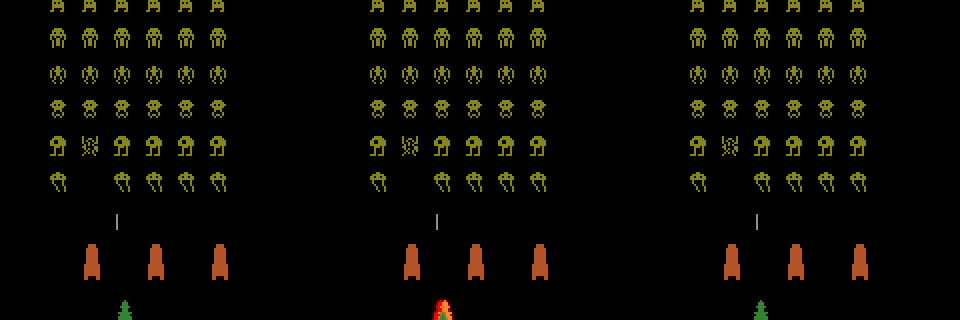}
        \caption{$a =$ \textit{MoveLeftAndFire}, $a'=$ \textit{Fire}.}
    \end{subfigure}%
    \hfill
    \begin{subfigure}{0.49\textwidth}
        \centering
        \includegraphics[width=\textwidth]{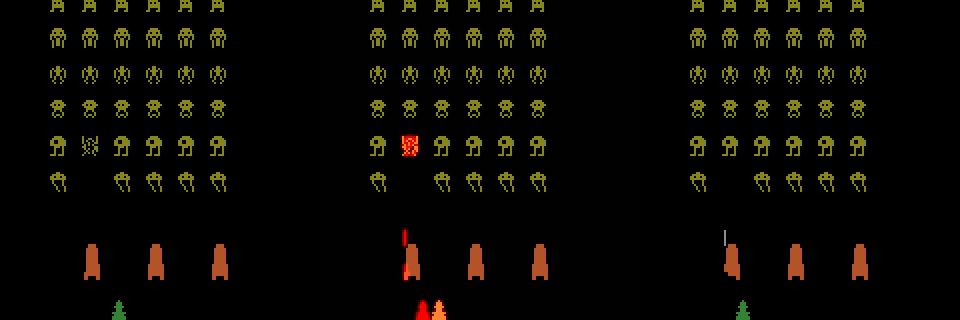}
        \caption{$a =$ \textit{MoveRightAndFire}, $a'=$ \textit{MoveLeft}.}
    \end{subfigure}%
    ~ 
    \begin{subfigure}{0.49\textwidth}
        \centering
        \includegraphics[width=\textwidth]{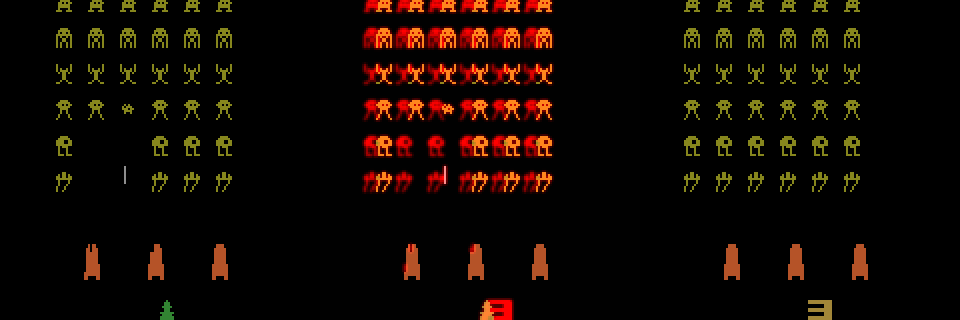}
        \caption{$a =$ \textit{MoveRightAndFire}, $a'=$ \textit{MoveLeft}.}
    \end{subfigure}%
    \hfill
    \begin{subfigure}{0.49\textwidth}
        \centering
        \includegraphics[width=\textwidth]{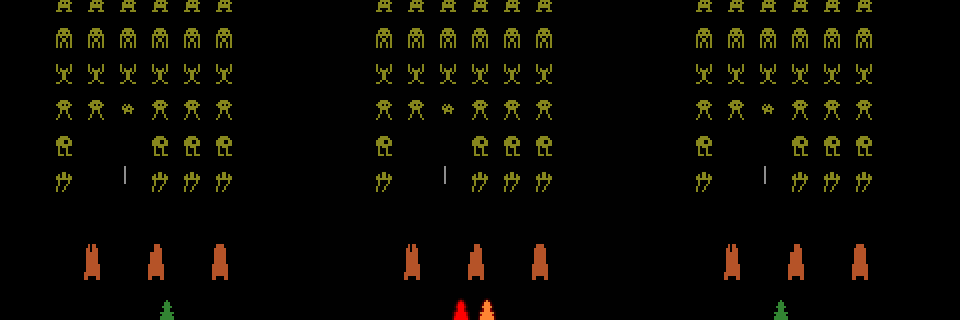}
        \caption{$a =$ \textit{MoveRightAndFire}, $a'=$ \textit{MoveLeftAndFire}.}
    \end{subfigure}%
    ~ 
    \begin{subfigure}{0.49\textwidth}
        \centering
        \includegraphics[width=\textwidth]{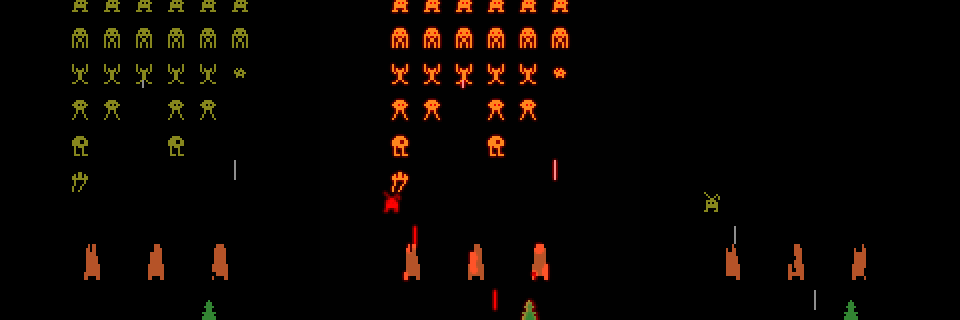}
        \caption{$a =$ \textit{MoveLeftAndFire}, $a'=$ \textit{Fire}.}
    \end{subfigure}%
    \hfill
    \begin{subfigure}{0.49\textwidth}
        \centering
        \includegraphics[width=\textwidth]{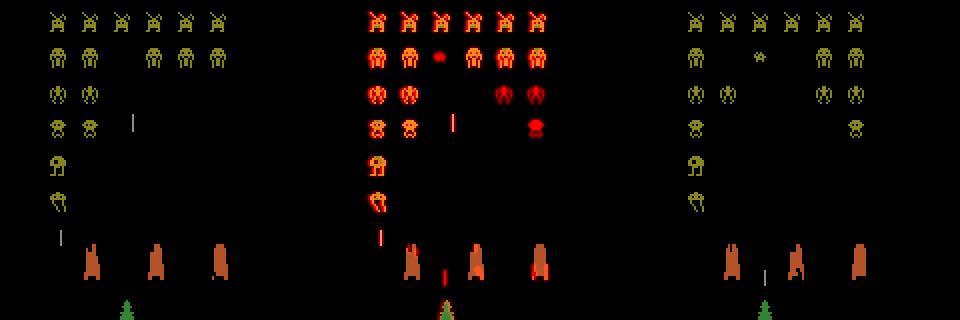}
        \caption{$a =$ \textit{MoveLeftAndFire}, $a'=$ \textit{MoveRight}.}
    \end{subfigure}%
    ~ 
    \begin{subfigure}{0.49\textwidth}
        \centering
        \includegraphics[width=\textwidth]{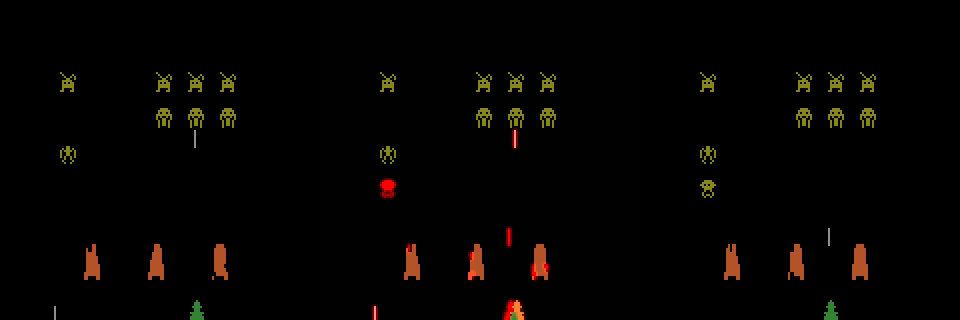}
        \caption{$a =$ \textit{Fire}, $a'=$ \textit{MoveLeftAndFire}.}
    \end{subfigure}%
    \hfill
    \begin{subfigure}{0.49\textwidth}
        \centering
        \includegraphics[width=\textwidth]{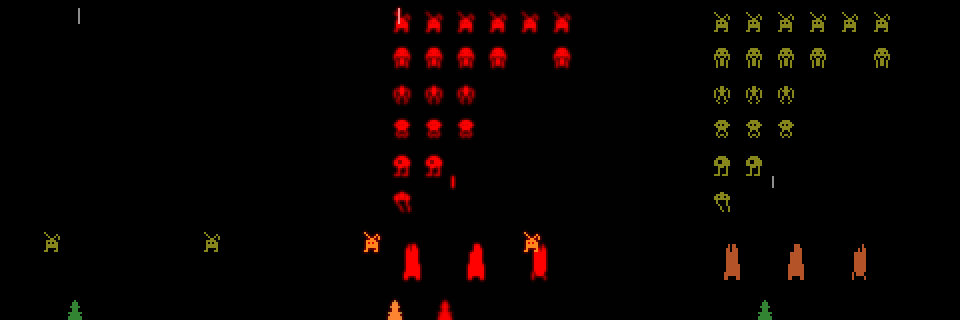}
        \caption{$a =$ \textit{MoveLeftAndFire}, $a'=$ \textit{MoveRightAndFire}.}
    \end{subfigure}%
    ~ 
    \caption{Representative counterfactuals for the nearest neighbor ablation. For each image: (\textbf{Left}) The original state where the agent took action $a$. (\textbf{Center}) The difference mask between the reconstructed state and the counterfactual state applied as red highlights. (\textbf{Right}) The counterfactual state where the agent took action $a'$. }
    \label{fig:nearest_neighbors}
\end{figure*}

\subsection{User Study Details}

We evaluate our counterfactual states through a user study with participants who were not experts in machine learning. Approximately half were undergraduates and the others were from the community. 80\% were between the ages of 18-30, 10\% were 30-50,  and the other 10 50-60. 
We did not use Mechanical Turk to perform the user study, and instead, participants came into our lab and did the study in person. This was done because it was critical that the participants paid close attention to all the instructions. We found that without having a guided in-person tutorial, users were confused with the explanation as counterfactuals are an esoteric topic for most non-experts. Also we found that by having someone run the study, participants did not try to answer the questions as quickly as possible, as is prone to happen on Turk. 

Our study consisted of 6 sections. Participants played the Atari 2600 video game Space Invaders for 5 minutes. 
For the second section, participants rated the realism of 30 randomly ordered game images on a Likert scale from 1 to 6.
\begin{enumerate}
\item
Completely fake.
\item
Most parts fake.
\item
More than half fake.
\item
More than half real.
\item
Most parts real.
\item
Completely real.
\end{enumerate}
The images were an even mix of images generated by three different sources: 10 from the actual game, 10 from our counterfactual method, and 10 from our ablation experiment. These images were randomly shuffled for each users.
The real images and the counterfactual images are the same images used for explanations in the next part of the study and are shown in figure \ref{fig:user_study_images} as the left and right states.  The ablated images, which users found fake, are shown in \ref{fig:ablated_realism_study}.

\begin{figure*}
    \centering
    \includegraphics[width=\linewidth]{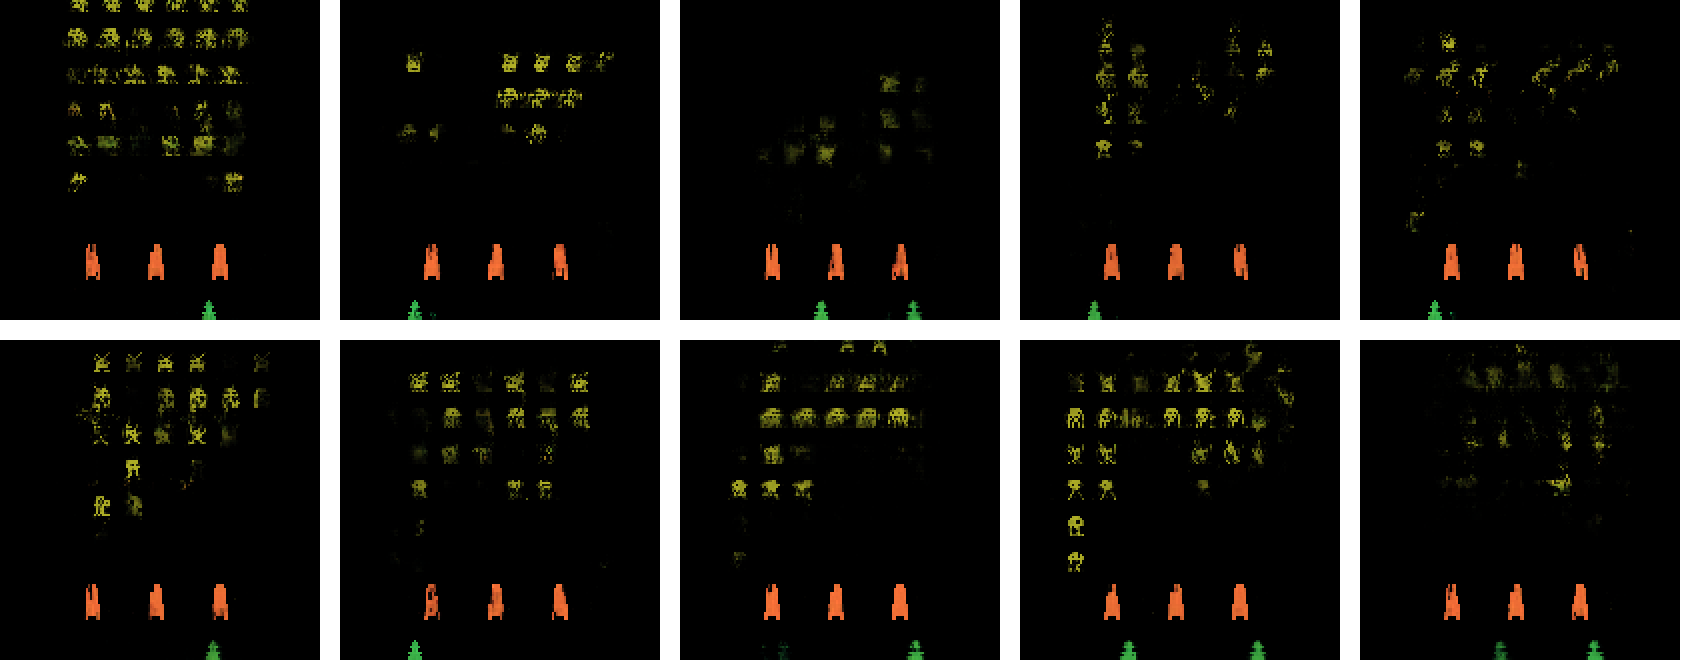}
    \caption{The 10 counterfactual images generated by our ablated model used in the user study to determine realism.}

    \label{fig:ablated_realism_study}
\end{figure*}

In the 3rd section, we showed users a video of an agent playing one sequence of Space Invaders where the agent clears the screen of all enemies. We then asked the following question: \textit{``On a scale of 1 to 6, to what extent do you feel like you understand how the AI is making decisions?''}
\begin{enumerate}
\item
I  don't feel like I know how it's making any decisions.
\item
I  don't feel like I know how it's making most of its decisions.
\item
I  don't feel like I know how it's making some of its decisions.
\item
I feel like I know how it's making  some of  its decisions.
\item
I feel like I know how it's making  most of  its decisions.
\item
I feel like I know how it's making  all  of its decisions.
\end{enumerate}

In the fourth section, we ran a tutorial for the users to explain what a counterfactual state is, how we could ask the agent such a query, and how the agent would respond. Figure \ref{fig:tutorial} shows the precise layout we used for displaying the counterfactual states, but for the tutorial we hid all of the interface, and revealed a single element from the table one step at a time. The counterfactual used in the tutorial was hand selected and not used in the next section. We started showing only the question and the shell of the table that was to be filled in. We revealed one element at a time, starting with the "Original Screenshot" column, then the "Changed State", and lastly the "Highlights". We found that by explaining each part of the table with simply text was insufficient and left participants confused. We had participants follow along with a demonstrator, where the demonstrator would tell participants when to reveal the next element and how that element contributes to the explanation.

\begin{figure*}
    \centering
    \includegraphics[width=\linewidth]{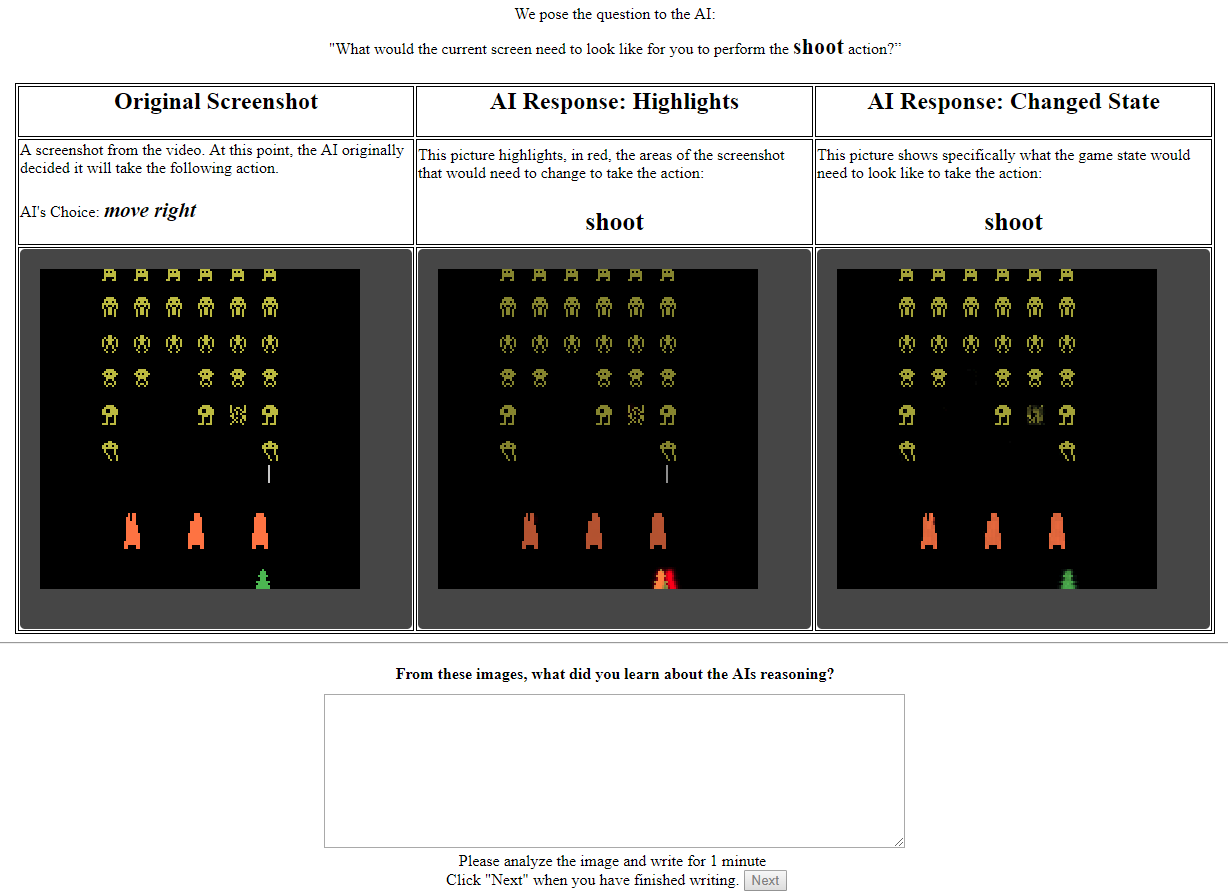}
    \caption{The user interface for explaining counterfactual states.}

    \label{fig:tutorial}
\end{figure*}

Though we had all 4 game frames available for the original and counterfactual state, we decided to only show the current time step to maintain simplicity. 
The center image titled ``AI Response: Highlights'' is an extra piece of information we decided to include to help participants find the change between the original state and the counterfactual state.

The Highlight images are created by taking the original output of our architecture %$G(E(s),\bm{\pi}(A(s)))$ and subtracting it from $G(E(s),\bm{\pi}(z^*))$
, taking the absolute difference between it and the counterfactual state to create a mask, applying a red Gaussian filter to that mask, and placing it on top of the original state. 

In the 5th section, we showed the users 10 counterfactual states displayed alongside the original query state and an image that highlights the changes as demonstrated in Figure \ref{fig:tutorial}. We chose the game images from the video we had shown previously. All 10 example explanations can been seen in Figure \ref{fig:user_study_images}.

To reiterate from before: the specific images, serving as query states for our counterfactuals, were chosen using a heuristic based on entropy, which has been used in the past for choosing key frames for establishing trust \cite{huang2018}. 
For diversity, if a key frame was selected, we do not allow images from the next two time-steps to be selected. 
Once a query state was selected, we selected the counterfactual action as the one that required the largest $L_2$ change between the original latent state $\bm{z}$ and the counterfactual latent state $\bm{z'}$ (ignoring the no-operation action). 
The counterfactual states were not hand-picked; rather, they were selected by ranking game images according to our heuristic and then selecting the counterfactual action according to the previous criterion.
For each counterfactual state generated, we asked the participant what they learned about the agent's decision making, and they answered in a free text response box. Here we present examples of each code:

\paragraph{Death:}
\textit{``...the ship dying changed its decision.''}
-- User 2091501, Example 3.

\paragraph{Barrier:}
\textit{``It does not want to move under the barricade but prefers to stay out and shoot.''}
-- User 2101304, Example 3.

\paragraph{Enemies:}
\textit{``The AI seems to know how the aliens move. It is anticipating the aliens' move to the right''}
-- User 2071601, Example 10.

\paragraph{Pose:}
\textit{``There are certain "remembered" locations of the AI where the shoot action was most advantageous, i.e. the spot highlighted in red...''}
-- User 2061401, Example 7.

\paragraph{Shot:}
\textit{``The AI is attempting to avoid being shot. It can see the position of the "laser" relative to itself... ''} -- User 2071601, Example 1.

\paragraph{No Insight:}
\textit{``This instance seems like a glitch to me I can't make sense of it.''} -- User 2101504, Example 3.

In the 6th and final section, we repeated the question from section 3, ``On a scale of 1 to 6, to what extent do you feel like you understand how the AI is making decisions?'' and we also asked ``In regards to your understanding of the AI, which images were most useful?'' where the users could respond with the highlights (11), the changed state (6), both (12), or neither (1).

\begin{figure*}[t]
    \centering
    \begin{subfigure}{0.49\textwidth}
        \centering
        \includegraphics[width=\textwidth]{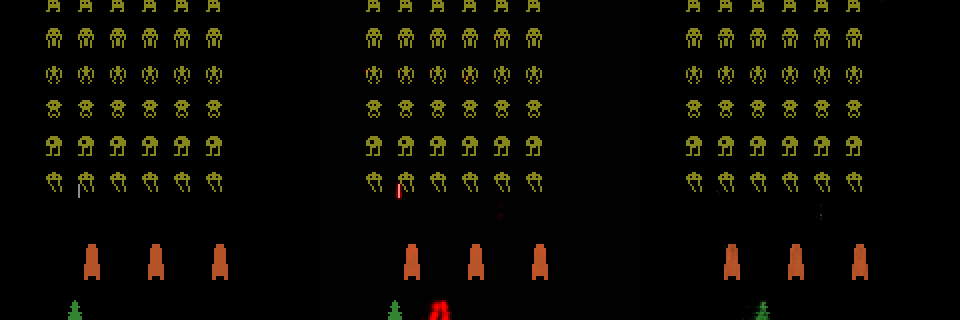}
        \caption{$a =$ \textit{MoveRightAndFire}, $a'=$ \textit{MoveLeft}.}
    \end{subfigure}%
    ~ 
    \begin{subfigure}{0.49\textwidth}
        \centering
        \includegraphics[width=\textwidth]{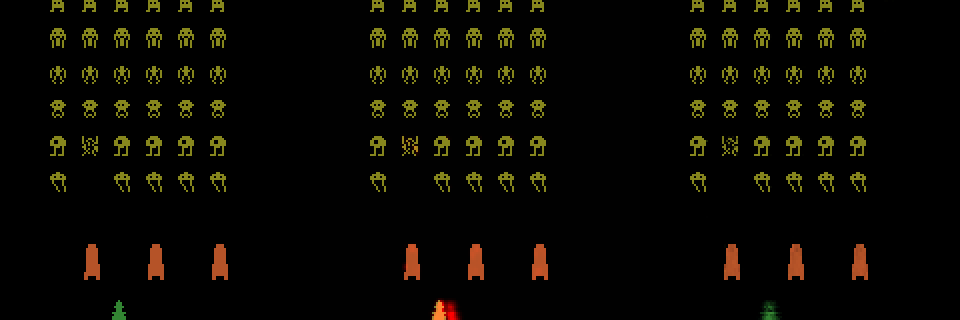}
        \caption{$a =$ \textit{MoveRightAndFire}, $a'=$ \textit{MoveLeft}.}
    \end{subfigure}%
    \hfill
    \begin{subfigure}{0.49\textwidth}
        \centering
        \includegraphics[width=\textwidth]{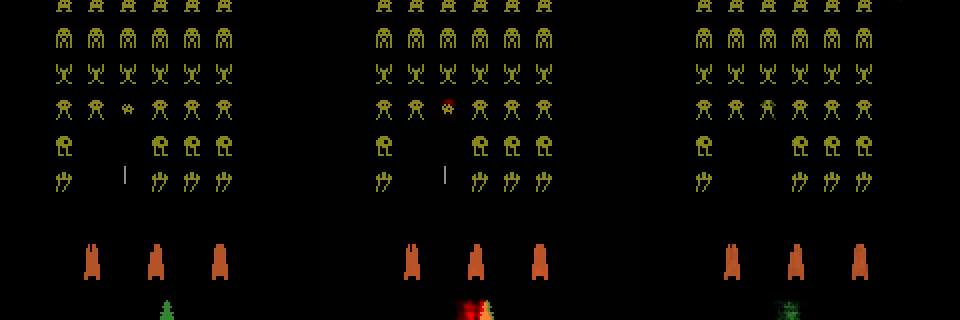}
        \caption{$a =$ \textit{MoveRightAndFire}, $a'=$ \textit{MoveLeft}.}
    \end{subfigure}%
    ~ 
    \begin{subfigure}{0.49\textwidth}
        \centering
        \includegraphics[width=\textwidth]{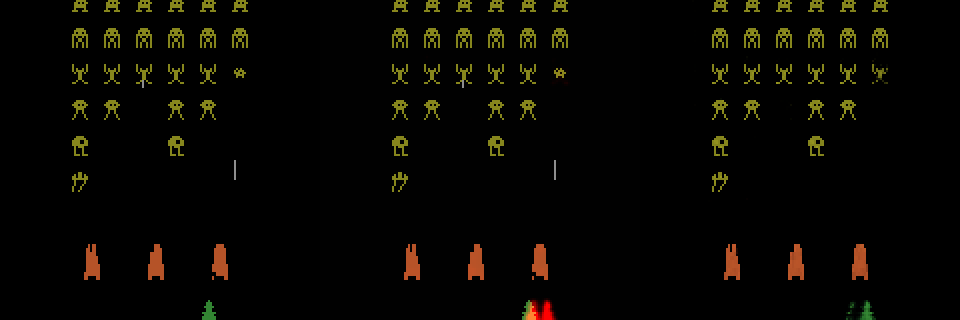}
        \caption{$a =$ \textit{MoveLeftAndFire}, $a'=$ \textit{Fire}.}
    \end{subfigure}%
    \hfill
    \begin{subfigure}{0.49\textwidth}
        \centering
        \includegraphics[width=\textwidth]{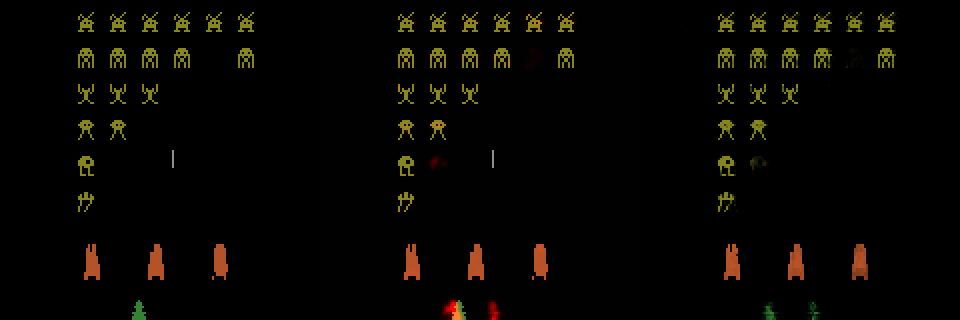}
        \caption{$a =$ \textit{MoveLeftAndFire}, $a'=$ \textit{MoveRightAndFire}.}
    \end{subfigure}%
    ~ 
    \begin{subfigure}{0.49\textwidth}
        \centering
        \includegraphics[width=\textwidth]{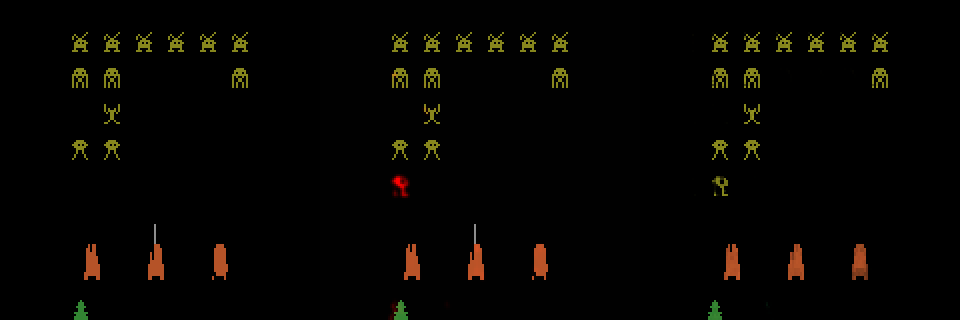}
        \caption{$a =$ \textit{MoveRight}, $a'=$ \textit{Fire}.}
    \end{subfigure}%
    \hfill
    \begin{subfigure}{0.49\textwidth}
        \centering
        \includegraphics[width=\textwidth]{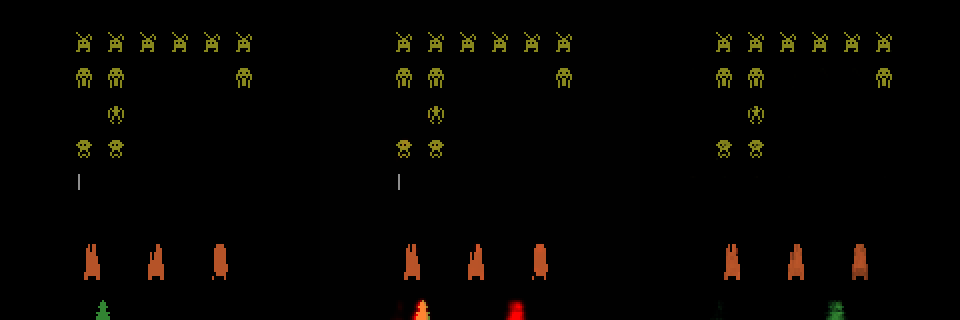}
        \caption{$a =$ \textit{MoveRight}, $a'=$ \textit{Fire}.}
    \end{subfigure}%
    ~ 
    \begin{subfigure}{0.49\textwidth}
        \centering
        \includegraphics[width=\textwidth]{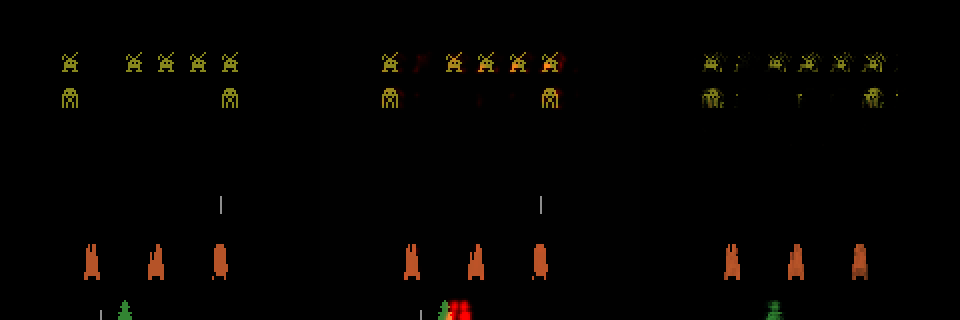}
        \caption{$a =$ \textit{MoveRight}, $a'=$ \textit{MoveLeft}.}
    \end{subfigure}%
    \hfill
    \begin{subfigure}{0.49\textwidth}
        \centering
        \includegraphics[width=\textwidth]{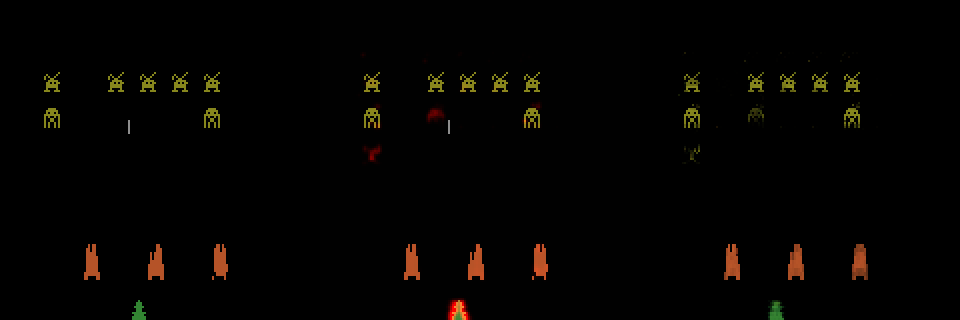}
        \caption{$a =$ \textit{MoveRight}, $a'=$ \textit{Fire}.}
    \end{subfigure}%
    ~ 
    \begin{subfigure}{0.49\textwidth}
        \centering
        \includegraphics[width=\textwidth]{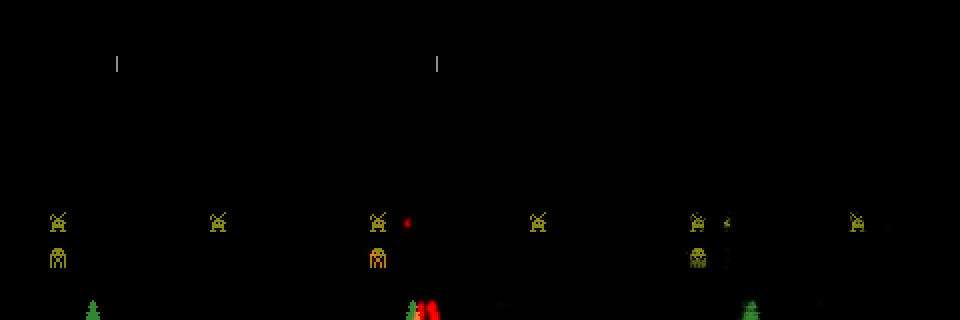}
        \caption{$a =$ \textit{MoveLeftAndFire}, $a'=$ \textit{MoveRight}.}
    \end{subfigure}%
    \caption{The 10 sets of explanation images shown to the users. For each image: (\textbf{Left}) The original state where the agent took action $a$. (\textbf{Center}) The difference mask between the reconstructed state and the counterfactual state applied as red highlights. (\textbf{Right}) The counterfactual state where the agent took action $a'$. }
    \label{fig:user_study_images}
\end{figure*}

%We then showed the users a video of the agent playing a round and asked the them to rate their understanding of the agent before and after seeing our counterfactual explanations. 
%With a similar Likert scale, 1 being not understanding how the agent makes decisions, 6 being complete understanding on all deicsions
%We found 15 users' understanding increased, 8 decreased, and 7 stayed the same.

%We showed the users 10 counterfactual explanations arrayed in a similar fashion to the images above. For every explanation, we asked the user what they learned about the agent's decision making. We coded all of this free text input, which could coarsely be seperated into: "the user gained insight into the agent's decision making" or "the user did not gain insight", where insight is defined as the user noting the agent's understanding of a game concept, and the opposite is defined as the user stating they are confused or simply transcribing the image.
